# Supplementary material for: Verifying OpenJDK's LinkedList using KeY
Source: arXiv:1911.04195 source file (2019-11-11)
Supplement: Supplementary file 1 [file 1_bug_reports.tex]

\section{Bug Report}

Over the years, 877 bugs are reported in the official OpenJDK bug tracker\footnote{\footnote{\url{https://bugs.openjdk.java.net/browse/JDK-8218584?jql=project\%20in\%20(JDK)\%20AND\%20component\%20in\%20(core-libs)\%20AND\%20Subcomponent\%20in\%20(java.util\%3Acollections)}}}. We also submitted a bug report, describing the issues encountered and proposes our solution. This report is attached below.

The JVM arguments for test cases 1, 2 and 3 are:

\begin{verbatim}
-Xms65G -Xmx65G -Xloggc:TestCase1_65G_OOP_gc.log
-XX:ObjectAlignmentInBytes=32 -XX:+PrintClassHistogramBeforeFullGC
-XX:+PrintGC -XX:+PrintGCDateStamps -XX:+PrintGCDetails
-XX:+PrintGCTimeStamps  -XX:+UseCompressedClassPointers
-XX:+UseCompressedOops -XX:+UseG1GC
\end{verbatim}
 
\noindent The JVM arguments for test cases 4 and 5 are:

\begin{verbatim}
-Xms167G -Xmx167G -Xloggc:TestCase4_167G_OOP_gc.log
-XX:+PrintClassHistogramBeforeFullGC -XX:+PrintGC
-XX:+PrintGCDateStamps -XX:+PrintGCDetails -XX:+PrintGCTimeStamps
\end{verbatim}
