# Supplementary material for: Verifying OpenJDK's LinkedList using KeY
Source: arXiv:1911.04195 source file (2019-11-11)
Supplement: Supplementary file 2 [file 2_impact_analysis.tex]

\section{Impact Analysis}\label{sec:impact}
Consequential problems (in standard library)

Qualitative analysis of Maven repositories
