# Supplementary material for: Verifying OpenJDK's LinkedList using KeY
Source: arXiv:1911.04195 source file (2019-11-11)
Supplement: Supplementary file 3 [file 4_jml_specs.tex]

\section{JML Specifications}\label{sec:all-specs}
A complete source view of \texttt{BoundedLinkedList} with all annotations follows. Since KeY does not support generics, this has been removed. We leave out comments that are otherwise present in the original to save space. We also leave out those methods that were not specified and proven correct. \texttt{BoundedLinkedList} is based on JDK8, version jdk8-b132. This version is of 2014-03-04 as found on \url{https://hg.openjdk.java.net/jdk8/jdk8/jdk/}.

\begin{framed}
\inputminted[breaklines,linenos,fontsize=\scriptsize,tabsize=2]{jml.py:JMLLexer -x}{\snippet{BoundedLinkedList.java}}
\end{framed}
